# Supplementary material for: Improving Visual Recognition with Hyperbolical Visual Hierarchy Mapping
Source: arXiv:2404.00974 source file (2024-04-01)
Supplement: Supplementary file 1 [file algorithm.tex]

\SetKwInput{KwRequire}{Require}
\label{sec:alg}
\vspace{-4pt}
\begin{algorithm}
    \caption{VHM Training.}
    \label{al_ppl}
    \LinesNumbered
    \KwRequire{The pre-trained image encoder $\mathcal{F}$, hierarchy decomposition module $\mathcal{D}$, and hierarchy encoder $\mathcal{G}$}
    \KwRequire{Initial level semantic seed distribution $\{\mathcal{N}(\mu_{c^{1}_{k}}, \sigma_{c^{1}_{k}})\}_{k=1}^{N}$ are randomly initialized}
    \KwRequire{Hyperbolic spaces \(\mathbb{L}\) initialized with curvature \(c=1\)}
    \While{Training}{
        Draw a mini-batch (\(I\), \(y\)).\\
        Sample initial semantic seeds \(\mathbf{c}^{1}\) from \(\{(\mu_{c^{1}_{k}}, \sigma_{c^{1}_{k}})\}_{k=1}^{N}\),\\
        Compute $v=\mathcal{F}(I)$ and semantic nodes \(\mathbf{s}^{1} = \mathcal{D}(v_{map}, \mathbf{c}^{1} )\) \\
        set \(l-1\) level as initial level\\
        \For{l to L}{
            Compute \(\{\mathcal{N}(\mu_{c^{l}_{k}}, \sigma_{c^{l}_{k}})\}_{k=1}^{N_{l}}\) according to Eq. (\red{})\\
            Sample \(\mathbf{c}^{l}\) from \(\{\mathcal{N}(\mu_{c^{l}_{k}}, \sigma_{c^{l}_{k}})\}_{k=1}^{N_{l}}\) according to Eq. (\red{})\\
            Compute \(l\) level semantic nodes \(\mathbf{s}^{l}\) according to Eq. (\red{})\\
            Compute representative semantic nodes \(\mathbf{s}^{l}_{k}\) according to Eq. (\red{})
        }
        \\
        Let $\boldsymbol{w}_{c}=\left[w_c^1,...,w_c^K\right] $\\
        Compute $\mathcal{L}_{div}$ according to Eq. (5)\\
        Compute $\boldsymbol{\sigma}_c^k=\mathcal{M}(w_{c}^k, v)$\\
        Compute $p(z|\boldsymbol{w}_c)$ according to Eq. (8)\\
        Compute $\mu(\boldsymbol{w}_c)$ and $\sigma(\boldsymbol{w}_c)$ according to Eq. (16), (17)\\
        Sample text embedding $\boldsymbol{z}_c$ from $p(z|\boldsymbol{w}_c)$\\
        Compute uncertainty $\log\sigma^2$ according to Eq. (18)\\
        Compute $\mathcal{L}_{KL}$ according to Eq. (12)\\
        Compute $\mathcal{L}_{pixel}$ according to Eq. (10)\\
        Compute $\mathcal{L}_{prob}$ according to Eq. (11)\\
        Compute total loss $\mathcal{L}$ according to Eq. (13)\\
        Update $\mathbf{P}$ and $\mathcal{M}$ by gradient descent\\}
\end{algorithm}
