# Supplementary material for: Improving Visual Recognition with Hyperbolical Visual Hierarchy Mapping
Source: arXiv:2404.00974 source file (2024-04-01)
Supplement: Supplementary file 2 [file compile_table.tex]

\begin{table}[ht]
    \centering
    \begin{subtable}[t]{\linewidth}
        \centering
        \caption{\textbf{Quantitative results of image classification on ImageNet-1K.} with Swin-Tiny model~\cite{swin}}
{\scriptsize
\label{tab:addlabel}
\begin{tblr}{
  colspec = {Q[367]Q[190]Q[171]Q[154]},
  cells = {c},
  row{4} = {LinkWater},
  cell{1}{1} = {r=2}{},
  hline{1,3,5} = {-}{},
}
Model                 & Params & FLOPs & Top-1         \\
                      & (M)    & (G)   & (\%)          \\
Swin-T                & 28.3   & 4.6   & 81.2          \\
\textbf{VHM}Swin-T & 29.5   & 4.9   & \textbf{83.4} 
\end{tblr}}

 % 첫 번째 테이블
    \end{subtable}
    \hfill % 테이블 사이의 간격을 조정합니다.
    \begin{subtable}[t]{\linewidth}
        \centering
        \caption{\textbf{Quantitative results of object section and instance segmentation on COCO.} with Swin-Tiny model~\cite{swin}}
{\scriptsize
\label{tab:addlabel}
\begin{tblr}{
  colspec = {Q[330]Q[130]Q[130]Q[130]Q[130]},
  cells = {c},
  row{4} = {LinkWater},
  cell{1}{1} = {r=2}{},
  cell{1}{4} = {r=2}{},
  cell{1}{5} = {r=2}{},
  hline{1,3,5} = {-}{},
}
Model              & Params & FLOPs & $AP^b$        & $AP^m$        \\
                   & (M)    & (G)   &               &               \\
Swin-T             & 48     & 267   & 42.7          & 39.3          \\
\textbf{VHM}Swin-T & 50     & 270   & \textbf{43.5} & \textbf{39.9} 
\end{tblr}}
 % 두 번째 테이블
    \end{subtable}
    \hfill
    \begin{subtable}[t]{\linewidth}
        \centering
        \caption{\textbf{Quantitative results of semantic segmentation on ADE20K.} with Swin-Tiny model~\cite{swin}}
{\scriptsize
\label{tab:addlabel}
\begin{tblr}{
  colspec = {Q[350]Q[200]Q[130]Q[130]Q[130]},
  row{1} = {c},
  row{2} = {c},
  row{4} = {LinkWater},
  cell{1}{1} = {r=2}{},
  cell{1}{2} = {r=2}{},
  cell{1}{5} = {r=2}{},
  cell{3}{1} = {c},
  cell{3}{3} = {c},
  cell{3}{4} = {c},
  cell{3}{5} = {c},
  cell{4}{1} = {c},
  cell{4}{3} = {c},
  cell{4}{4} = {c},
  cell{4}{5} = {c},
  hline{1,3,5} = {-}{},
}
Model           & Method   & Params & FLOPs & mIoU          \\
                   &          & (M)    & (G)   &               \\
Swin-T             & UpderNet & 60     & 945.0 & 44.5          \\
\textbf{VHM}Swin-T & UpderNet & 62.1   & 948.3 & \textbf{46.8} 
\end{tblr}}
 % 세 번째 테이블
    \end{subtable}
\end{table}
