# Supplementary material for: Improving Visual Recognition with Hyperbolical Visual Hierarchy Mapping
Source: arXiv:2404.00974 source file (2024-04-01)
Supplement: Supplementary file 3 [file supple_cls.tex]

{\scriptsize
\label{tab:addlabel}
\begin{tblr}{
  colspec = {Q[367]Q[190]Q[171]Q[154]},
  cells = {c},
  row{4} = {LinkWater},
  cell{1}{1} = {r=2}{},
  hline{1,3,5} = {-}{},
}
Model                 & Params & FLOPs & Top-1         \\
                      & (M)    & (G)   & (\%)          \\
Swin-T                & 28.3   & 4.6   & 81.2          \\
\textbf{VHM}Swin-T & 29.5   & 4.9   & \textbf{83.4} 
\end{tblr}}
