# Supplementary material for: Improving Visual Recognition with Hyperbolical Visual Hierarchy Mapping
Source: arXiv:2404.00974 source file (2024-04-01)
Supplement: Supplementary file 4 [file supple_mask.tex]

{\scriptsize
\label{tab:addlabel}
\begin{tblr}{
  colspec = {Q[330]Q[130]Q[130]Q[130]Q[130]},
  cells = {c},
  row{4} = {LinkWater},
  cell{1}{1} = {r=2}{},
  cell{1}{4} = {r=2}{},
  cell{1}{5} = {r=2}{},
  hline{1,3,5} = {-}{},
}
Model              & Params & FLOPs & $AP^b$        & $AP^m$        \\
                   & (M)    & (G)   &               &               \\
Swin-T             & 48     & 267   & 42.7          & 39.3          \\
\textbf{VHM}Swin-T & 50     & 270   & \textbf{43.5} & \textbf{39.9} 
\end{tblr}}
