# Supplementary material for: Improving Visual Recognition with Hyperbolical Visual Hierarchy Mapping
Source: arXiv:2404.00974 source file (2024-04-01)
Supplement: Supplementary file 5 [file supple_seg.tex]

{\scriptsize
\label{tab:addlabel}
\begin{tblr}{
  colspec = {Q[350]Q[200]Q[130]Q[130]Q[130]},
  row{1} = {c},
  row{2} = {c},
  row{4} = {LinkWater},
  cell{1}{1} = {r=2}{},
  cell{1}{2} = {r=2}{},
  cell{1}{5} = {r=2}{},
  cell{3}{1} = {c},
  cell{3}{3} = {c},
  cell{3}{4} = {c},
  cell{3}{5} = {c},
  cell{4}{1} = {c},
  cell{4}{3} = {c},
  cell{4}{4} = {c},
  cell{4}{5} = {c},
  hline{1,3,5} = {-}{},
}
Model           & Method   & Params & FLOPs & mIoU          \\
                   &          & (M)    & (G)   &               \\
Swin-T             & UpderNet & 60     & 945.0 & 44.5          \\
\textbf{VHM}Swin-T & UpderNet & 62.1   & 948.3 & \textbf{46.8} 
\end{tblr}}
